# Supplementary material for: Contrastive Learning of Sociopragmatic Meaning in Social Media
Source: arXiv:2203.07648 source file (2023-05-25)
Supplement: Supplementary file 1 [file append_baselines.tex]

\subsection{Baselines} \label{subsec:app_baseline}
\textbf{(1) RB.} We fine-tune the original pre-trained RoBERTa, abbreviated as RB in our results Table~\ref{tab:main_result}, (without any further training) on downstream tasks with standard cross-entropy loss. \textbf{(2) MLM:} We continue pre-training RoBERTa on our TweetEmoji-EN dataset with solely MLM objective as Eq.~\ref{eq:mlm_loss} shows, and then fine-tune the model on downstream tasks. \textbf{(3) Emoji-Based MLM:}~\citet{corazza2020hybrid} introduce an emoji-based MLM (E-MLM) to integrate emoji information into PLM giving masking priority to emojis in a given text. We train E-MLM on our TweetEmoji-EN dataset~\footnote{We create another version of TweetEmoji-EN that includes the original emojis in the tweets.} and evaluate on downstream tasks. \textbf{(4) SLP.} We first fine-tune the RoBERTa on the \textit{surrogate label prediction} task (emoji prediction) with cross-entropy loss in Eq.~\ref{eq:ce}, then fine-tune the obtained model on downstream tasks. 
\textbf{Supervised Contrastive Learning:} We also compare to state-of-the-art supervised contrastive fine-tuning frameworks. We take the original pre-trained RoBERTa and fine-tune it on each task with \textbf{(5) SCL}~\cite{gunel2020supervised} and \textbf{(6) LCL}~\cite{suresh2021not}, respectively. Both works combine supervised contrastive loss with standard cross-entropy as well as augmentation of the training data to construct positive pairs. We follow the augmentation technique used in~\citet{suresh2021not}, which replaces $30\%$ of words in the input sample with their synonyms in WordNet dictionary~\cite{miller1995wordnet}. \textbf{Self-Supervised Contrastive Learning.} We further pre-train RoBERTa on different recently proposed self-supervised contrastive learning frameworks. \textbf{(7) SimCSE-Self.}~\citep{gao2021simcse} introduce SimCSE where they produce a positive pair by applying different dropout masks on input text twice. We similarly acquire a positive pair using the same droput method. \textbf{(8) SimCSE-Distant.}~\citep{gao2021simcse} also propose a supervised SimCSE that utilizes gold NLI data, rather than dropout masking, to create positive pairs where an anchor is a premise and a positive sample is a entailment of the premise. %~\footnote{They also use a contradiction of a premise as a hard negative sample.} 
Hence, we adapt the supervised SimCSE framework to our distantly supervised data and construct positive pairs applying our epoch-wise re-pairing strategy. Specifically, each anchor has one positive sample that employs the same emoji as the anchor in a batch.%~\footnote{We leave the hard negative mining with distant supervision as a future work.} 
\footnote{Different from SCL loss, SimCSE-Distant still uses SSCL loss where each anchor only recognizes one paired sample as its positive. If there is another pair with the same emoji label, SimCSE-Distant considers them as negative samples. This is intended to employ surrogate labels as an instance-level data augmentation method similar to dropout.} \textbf{(9) Mirror-BERT.}~\cite{liu2021fast} construct Mirror-BERT by random span masking as well as different dropout masks. After the contrastive learning, sentence-encoder models are fine-tuned on downstream tasks with standard cross-entropy loss.

\textbf{(10) Weakly-supervised Contrastive Learning.} We simplify and adapt the WCL framework of~\citet{zheng2021weakly} to language: We first encode unlabelled tweets to sequence-level representation vectors using the hidden state of `[CLS]' token from the last layer of RoBERTa. All unlabelled tweets are clustered by applying $k$-means to their representation vectors. We then use the cluster IDs as weak labels to perform an SCL to pull the tweets assigned to the same cluster closer. Following~\citet{zheng2021weakly}, we also include an SSCL loss by augmenting the positive sample of an anchor using random span masking as well as dropout masking. We jointly optimize the SCL and SSCL losses in our implementation.%~\footnote{We acknowledge that this is simplified implementation of WCL. It is a future work how to learn language representation with weak supervision. }

%Namely, we compare to \textbf{SimCSE}~\cite{gao2021simcse} and \textbf{Mirror-BERT}~\cite{liu2021fast}. Both models are trained with self-supervised contrastive loss as Eq.~\ref{eq:selfcl} shows. SimCSE~\cite{gao2021simcse} produce a positive pair by applying different dropout masks on a input text twice. A positive pair in Mirror-BERT~\cite{liu2021fast} is constructed by random span masking as well as different dropout masks. SimCSE~\cite{gao2021simcse} also exploits labelled natural language inference (NLI) datasets to form positive pairs, which use a premise as anchor, entailment of the premise as its positive sample, and its contradiction as its negative sample. After the contrastive learning, sentence-encoder models are fine-tuned on downstream tasks with standard cross-entropy loss.
%%%%%%%%%%%%%%%%%%

\textbf{(11) Domain-specific pre-trained language model (BTw):} We further compare our method to the SoTA domain-specific pre-trained LM, BERTweet~\cite{nguyen-etal-2020-bertweet}. BERTweet was pre-trained on $850$M tweets with RoBERTa\textsubscript{Base} architecture. We download the pre-trained BERTweet checkpoint from Huggingface's Transformers~\cite{wolf2020transformers} library and fine-tune it on each downstream task with a standard cross-entropy loss.
